# Supplementary material for: Multi-Agent Trustworthy Consensus under Random Dynamic Attacks
Source: arXiv:2504.07189 source file (2025-04-09)
Supplement: Supplementary file 1 [file appendix.tex]

% !TEX root = Control of stochastic disease network games via influential individuals.tex

\section{Appendix}
\label{sec:app}

\subsection{Proof of Theorem \ref{thm_azuma_sum}}
We have the following result by Assumptions \ref{leg_ag}-\ref{mal_ag} and the properties of conditional expectations,
\begin{align}
    &\mathbb{E}(\alpha_{im}(t)-\alpha_{il}(t)  |\mathbf{f}_m(t-1)) \nonumber \\
    &=\mathbb{E}(\alpha_{im}(t)-\alpha_{il}(t)  |f_m(t)=1, \mathbf{f}_m(t-1)) \mathbb{P}(f_m(t)=1) \nonumber \\
    &+ \mathbb{E}(\alpha_{im}(t)-\alpha_{il}(t)  |f_m(t)=0, \mathbf{f}_m(t-1)) \mathbb{P}(f_m(t)=0) \nonumber \\
    &=(E_M-E_L) \mathbb{P}(f_m(t)=1) \nonumber
\end{align}
Using the Hoeffding's Lemma( Lemma \ref{lem_hoeff}) from the theorem statement, we have for any $\omega >0$, with the property $|\alpha_{im}(t)-\alpha_{il}(t)|\le 1$,
    \begin{align} \label{eq_hoeffding}
         \mathbb{E}(\exp(\omega (\alpha_{im}(t)-\alpha_{il}(t))))  |\mathbf{f}_m(t-1)) \nonumber \\
         &\hspace{-0.7 in} \le \exp(\omega (E_M-E_L) p_m(t) +\frac{1}{2} \omega^2). \nonumber
         %&+\exp(\omega (E_M-E_L)  p_m(t) +\frac{1}{2} \omega^2).
    \end{align}
Next, we also bound the exponential of random sum using the individual bounds on summands, 
    \begin{align}
        &\mathbb{E}(\exp(\omega  (\beta_{im}(t)-\beta_{il}(t) )))=\mathbb{E} (\prod_{k=0}^t \exp(\omega( \alpha_{im}(t)-\alpha_{il}(t))))\nonumber \\
        &= \sum_{\mathbf{f}_m(t-1) \in Supp 
        (\mathcal{F}(t-1))}\mathbb{E}(\prod_{k=0}^t \exp(\omega ( \alpha_{im}(t)-\alpha_{il}(t)))  | \mathbf{f}_m(t-1)) \nonumber \\
        &\times \mathbb{P} (\mathbf{f}_m(t-1)) \nonumber \\
        &=\sum_{\mathbf{f}_m(t-1) \in Supp 
        (\mathcal{F}(t-1))}\prod_{k=0}^t \mathbb{E}( \exp(\omega ( \alpha_{im}(t)-\alpha_{il}(t)))  | \mathbf{f}_m(t-1)) \nonumber\\
        &\times \mathbb{P} (\mathbf{f}_m(t-1)) \nonumber \\
        &\le \exp(\omega \sa{(E_M-E_L)} p_m(t) +\frac{1}{2} \omega^2) \mathbb{E}(\prod_{k=0}^{t-1} \exp(\omega u(k))) \nonumber.
  \end{align}
By reiterating the conditioning $\mathbf{f}_m(k-1)$ for each summand $\alpha_{im}(k)-\alpha_{il}(k)$ for the time steps, $k \in \{1,\cdots,t\}$, and using $p_m(0)$ for the time step $k=0$ as a lower bound on the initial attack probability $\mathbb{P}(f_m(0)=1)\ge p_m(0)$, we conclude,
\begin{align*}
    \mathbb{E}(\exp(\omega  (\beta_{im}(t)&-\beta_{il}(t) ))) \\
    &\le \exp(\omega (E_M-E_L) \sum_{k=0}^t p_m(t) +\frac{(t+1)}{2} \omega^2).
\end{align*}
Next, we derive a bound for the probability of the event by Markov's Inequality,
\begin{align*}
     & \mathbb{P} (  \beta_{im}(t)-\beta_{il}(t) >  (E_M-E_L) \sum_{k=0}^t p_m(t)+ q \sqrt{(t+1)} )\\
    %=&  \mathbb{P} ( \omega  g(t) > \omega ((t+1)\bar{u}+ q \sqrt{(t+1)} b ))\\
    =& \mathbb{P} ( \exp(\omega  (\beta_{im}(t)-\beta_{il}(t)))) >\\
    &\hspace{0.7 in }\exp(\omega (E_M-E_L) \sum_{k=0}^t p_m(t) + q \sqrt{(t+1)} ))) \\
    \le& \frac{\mathbb{E}(\exp(\omega (\beta_{im}(t)-\beta_{il}(t))))}{  \exp(\omega ( (E_M-E_L) \sum_{k=0}^t p_m(t)+ q \sqrt{(t+1)}))}\\
    \le &  \exp(\frac{(t+1)}{2}  \omega^2-\omega q \sqrt{(t+1)})
    %\frac{\exp((t+1)(\omega \bar{u} +\frac{1}{2} \omega^2  b^2))}{  \exp(\omega ((t+1)\bar{u}+ q \sqrt{(t+1)} b))}.
\end{align*}
Thus, replacing $\omega:= \frac{q}{\sqrt{t+1}} > 0$ provides the final result using $q>0$ and $t\ge0$.
